# Supplementary material for: GEB+: A Benchmark for Generic Event Boundary Captioning, Grounding and Retrieval
Source: arXiv:2204.00486 source file (2025-02-01)
Supplement: Supplementary file 5 [file video_content.tex]

\section{List of Contents in the Attached Supplementary Video}
\label{supp-sec:video}

In our submitted supplementary video, we illustrate four parts of our work: \textit{(1) Annotation Interface.} The interface we designed for our annotators. 
\textit{(2) Examples for Boundary Types.} Several samples of boundaries from our \textit{Kinetic-GEB+} dataset that due to different types of status changes. 
\textit{(3) Annotation Formats and Examples.} Visualized comparison among different format schemes of caption annotating, as well as the finalized raw annotation towards a sample video.
\textit{(4) Visualization of Predictions.} Examples of predictions generated by the best-performing method in Boundary Captioning, Boundary Grounding and Boundary Caption-Video Retrieval.
